# Supplementary material for: Scalable and Real-time Multi-Camera Vehicle Detection, Re-Identification, and Tracking
Source: arXiv:2204.07442 source file (2022-04-15)
Supplement: Supplementary file 1 [file appendices.tex]

\appendices
\section{Proof of the First Zonklar Equation}
Appendix one text goes here.

\section{}
Appendix two text goes here.
